# Supplementary material for: Applications and Challenges of Sentiment Analysis in Real-life Scenarios
Source: arXiv:2301.09912 source file (2023-01-24)
Supplement: Supplementary file 1 [file appendix01.tex]

\begin{frontmatter}
\chapter{Appendix title}%\label{chap:appa}
\end{frontmatter}

%\section{}\label{}
