# Supplementary material for: Applications and Challenges of Sentiment Analysis in Real-life Scenarios
Source: arXiv:2301.09912 source file (2023-01-24)
Supplement: Supplementary file 2 [file appendix02.tex]

\begin{frontmatter}
\chapter{Appendix title}%\label{chap:appb}
\end{frontmatter}
